# Supplementary material for: Leveraging power grid topology in machine learning assisted optimal power flow
Source: arXiv:2110.00306 source file (2022-04-26)
Supplement: Supplementary file 1 [file Supp.pdf]

# Leveraging power grid topology in machine learning assisted optimal power flow

Thomas Falconer and Letif Mones

## I. SUPPLEMENTARY MATERIAL

**T**O complete the set of our empirical results, we provide additional information regarding: (1) the training time statistics for local and extended global regression GNN models (Table I); (2) the number of parameters for global classification models with fixed topology (Table II); (3) the training time statistics for global classification models (Table III); (4) the MSE statistics of the test sets for global, local and extended global GNN regression models using the admittance matrix (Tables IV, V); and lastly (5) the number of parameters for global classification models with varying topology (Table VI).

TABLE I

TRAINING TIME STATISTICS (MEAN AND TWO-SIDED 95% CONFIDENCE INTERVALS) FOR LOCAL AND EXTENDED GLOBAL REGRESSION GNN MODELS

| Case         | Training time ( $\times 10^2$ s)            |                                             |                                             |                                              |                                              |                                              |
|--------------|---------------------------------------------|---------------------------------------------|---------------------------------------------|----------------------------------------------|----------------------------------------------|----------------------------------------------|
|              | $\mathcal{M}_{\text{local-3}}^{\text{GCN}}$ | $\mathcal{M}_{\text{local-3}}^{\text{CHC}}$ | $\mathcal{M}_{\text{local-3}}^{\text{GAT}}$ | $\mathcal{M}_{\text{global-4}}^{\text{GCN}}$ | $\mathcal{M}_{\text{global-4}}^{\text{CHC}}$ | $\mathcal{M}_{\text{global-4}}^{\text{GAT}}$ |
| 24-ieee-rtts | $2.98 \pm 0.49$                             | $12.95 \pm 1.76$                            | $6.30 \pm 1.38$                             | $8.25 \pm 1.55$                              | $14.92 \pm 2.25$                             | $10.03 \pm 1.65$                             |
| 30-ieee      | $2.57 \pm 0.41$                             | $10.22 \pm 1.17$                            | $6.54 \pm 1.31$                             | $9.57 \pm 2.36$                              | $15.86 \pm 1.72$                             | $9.79 \pm 1.63$                              |
| 39-epri      | $2.60 \pm 0.54$                             | $11.03 \pm 0.91$                            | $4.21 \pm 0.69$                             | $13.18 \pm 2.14$                             | $15.60 \pm 2.24$                             | $12.92 \pm 1.91$                             |
| 57-ieee      | $2.47 \pm 0.77$                             | $9.47 \pm 0.71$                             | $5.24 \pm 1.07$                             | $9.74 \pm 1.31$                              | $10.30 \pm 2.60$                             | $10.87 \pm 1.92$                             |
| 73-ieee-rtts | $6.44 \pm 0.88$                             | $17.77 \pm 3.08$                            | $12.12 \pm 3.67$                            | $11.58 \pm 1.69$                             | $23.40 \pm 3.17$                             | $19.56 \pm 5.16$                             |
| 118-ieee     | $4.72 \pm 0.72$                             | $12.75 \pm 1.60$                            | $9.44 \pm 1.65$                             | $9.85 \pm 1.07$                              | $6.79 \pm 0.77$                              | $17.46 \pm 5.86$                             |
| 162-ieee-dtc | $4.91 \pm 0.70$                             | $16.81 \pm 2.60$                            | $10.05 \pm 1.52$                            | $7.49 \pm 0.88$                              | $4.58 \pm 0.29$                              | $11.64 \pm 2.33$                             |
| 300-ieee     | $11.60 \pm 2.52$                            | $15.42 \pm 1.18$                            | $20.00 \pm 4.91$                            | $16.92 \pm 1.68$                             | $8.40 \pm 0.43$                              | $19.86 \pm 6.88$                             |
| 588-sdet     | $43.33 \pm 9.31$                            | $27.33 \pm 2.18$                            | $75.15 \pm 9.95$                            | $39.04 \pm 4.37$                             | $16.67 \pm 0.83$                             | $34.38 \pm 8.83$                             |

TABLE II

NUMBER OF PARAMETERS FOR GLOBAL CLASSIFICATION MODELS (FIXED TOPOLOGY)

| Case         | # of parameters                               |                                               |                                              |                                              |                                              |                                             |                                             |
|--------------|-----------------------------------------------|-----------------------------------------------|----------------------------------------------|----------------------------------------------|----------------------------------------------|---------------------------------------------|---------------------------------------------|
|              | $\mathcal{M}_{\text{global-3}}^{\text{FCNN}}$ | $\mathcal{M}_{\text{global-1}}^{\text{FCNN}}$ | $\mathcal{M}_{\text{global-4}}^{\text{CNN}}$ | $\mathcal{M}_{\text{global-3}}^{\text{GCN}}$ | $\mathcal{M}_{\text{global-3}}^{\text{CHC}}$ | $\mathcal{M}_{\text{global-3}}^{\text{SC}}$ | $\mathcal{M}_{\text{global-3}}^{\text{GC}}$ |
| 24-ieee-rtts | 3443                                          | 833                                           | 877                                          | 1034                                         | 1514                                         | 1674                                        | 1194                                        |
| 30-ieee      | 3643                                          | 244                                           | 720                                          | 359                                          | 839                                          | 999                                         | 519                                         |
| 39-epri      | 8120                                          | 1659                                          | 1617                                         | 1075                                         | 1555                                         | 1715                                        | 1235                                        |
| 57-ieee      | 13301                                         | 1150                                          | 1398                                         | 815                                          | 1295                                         | 1455                                        | 975                                         |
| 73-ieee-rtts | 30251                                         | 7203                                          | 6125                                         | 7095                                         | 7575                                         | 7735                                        | 7255                                        |
| 118-ieee     | 63807                                         | 9954                                          | 9366                                         | 10712                                        | 12536                                        | 13144                                       | 11320                                       |
| 162-ieee-dtc | 128323                                        | 24050                                         | 21974                                        | 24808                                        | 26632                                        | 27240                                       | 25416                                       |
| 300-ieee     | 494219                                        | 114791                                        | 107739                                       | 115549                                       | 117373                                       | 117981                                      | 116157                                      |
| 588-sdet     | 1460783                                       | 171842                                        | 166590                                       | 176688                                       | 178512                                       | 179120                                      | 177296                                      |
| 1354-pegase  | 7486643                                       | 734139                                        | 724971                                       | 734897                                       | 736721                                       | 737329                                      | 735505                                      |
| 2853-sdet    | 43369442                                      | 9690486                                       | 9619758                                      | 9759164                                      | 9760988                                      | 9761596                                     | 9759772                                     |

TABLE III

TRAINING TIME STATISTICS (MEAN AND TWO-SIDED 95% CONFIDENCE INTERVALS) FOR GLOBAL CLASSIFICATION MODELS

| Case         | Training time ( $\times 10^2$ s)              |                                               |                                              |                                              |                                              |                                             |                                             |
|--------------|-----------------------------------------------|-----------------------------------------------|----------------------------------------------|----------------------------------------------|----------------------------------------------|---------------------------------------------|---------------------------------------------|
|              | $\mathcal{M}_{\text{global-3}}^{\text{FCNN}}$ | $\mathcal{M}_{\text{global-1}}^{\text{FCNN}}$ | $\mathcal{M}_{\text{global-4}}^{\text{CNN}}$ | $\mathcal{M}_{\text{global-3}}^{\text{GCN}}$ | $\mathcal{M}_{\text{global-3}}^{\text{CHC}}$ | $\mathcal{M}_{\text{global-3}}^{\text{SC}}$ | $\mathcal{M}_{\text{global-3}}^{\text{GC}}$ |
| 24-ieee-rtts | $0.55 \pm 0.08$                               | $4.21 \pm 0.02$                               | $0.79 \pm 0.05$                              | $9.14 \pm 2.29$                              | $10.36 \pm 1.46$                             | $7.87 \pm 0.62$                             | $10.50 \pm 1.62$                            |
| 30-ieee      | $0.36 \pm 0.04$                               | $3.87 \pm 0.44$                               | $0.96 \pm 0.14$                              | $5.23 \pm 1.22$                              | $11.35 \pm 1.49$                             | $7.64 \pm 1.71$                             | $8.32 \pm 1.35$                             |
| 39-epri      | $0.51 \pm 0.06$                               | $3.32 \pm 0.48$                               | $0.70 \pm 0.14$                              | $14.50 \pm 2.71$                             | $11.81 \pm 1.37$                             | $9.36 \pm 1.44$                             | $10.94 \pm 1.68$                            |
| 57-ieee      | $0.20 \pm 0.02$                               | $1.98 \pm 0.73$                               | $0.49 \pm 0.04$                              | $9.29 \pm 1.79$                              | $4.96 \pm 0.45$                              | $6.37 \pm 1.10$                             | $5.61 \pm 0.54$                             |
| 73-ieee-rtts | $0.27 \pm 0.03$                               | $4.44 \pm 0.16$                               | $1.06 \pm 0.30$                              | $12.92 \pm 2.53$                             | $10.71 \pm 1.42$                             | $9.45 \pm 1.52$                             | $8.99 \pm 1.22$                             |
| 118-ieee     | $0.20 \pm 0.01$                               | $1.85 \pm 0.40$                               | $0.59 \pm 0.10$                              | $15.21 \pm 4.01$                             | $4.62 \pm 0.28$                              | $5.05 \pm 0.25$                             | $4.36 \pm 0.39$                             |
| 162-ieee-dtc | $0.18 \pm 0.01$                               | $0.81 \pm 0.09$                               | $0.52 \pm 0.05$                              | $7.86 \pm 0.87$                              | $3.37 \pm 0.18$                              | $4.37 \pm 0.41$                             | $3.44 \pm 0.19$                             |
| 300-ieee     | $0.15 \pm 0.00$                               | $0.58 \pm 0.02$                               | $0.34 \pm 0.03$                              | $5.29 \pm 0.53$                              | $3.44 \pm 0.11$                              | $4.53 \pm 0.23$                             | $2.81 \pm 0.15$                             |
| 588-sdet     | $0.14 \pm 0.00$                               | $0.50 \pm 0.02$                               | $0.23 \pm 0.01$                              | $4.00 \pm 0.41$                              | $3.77 \pm 0.07$                              | $5.05 \pm 0.19$                             | $2.94 \pm 0.10$                             |
| 1354-pegase  | $0.27 \pm 0.00$                               | $0.50 \pm 0.02$                               | $0.20 \pm 0.00$                              | $2.61 \pm 0.13$                              | $4.52 \pm 0.09$                              | $7.07 \pm 0.17$                             | $2.82 \pm 0.08$                             |
| 2853-sdet    | $1.32 \pm 0.01$                               | $0.65 \pm 0.02$                               | $0.40 \pm 0.01$                              | $8.53 \pm 0.19$                              | $12.61 \pm 0.11$                             | $17.26 \pm 0.44$                            | $9.28 \pm 0.12$                             |

TABLE IV

MSE STATISTICS (MEAN AND TWO-SIDED 95% CONFIDENCE INTERVALS) OF THE TEST SETS FOR GLOBAL GNN REGRESSION MODELS USING ADMITTANCE MATRIX (FIXED TOPOLOGY)

| Case         | MSE ( $\times 10^{-3}$ )                      |                                              |                                              |                                             |                                             |                                              |
|--------------|-----------------------------------------------|----------------------------------------------|----------------------------------------------|---------------------------------------------|---------------------------------------------|----------------------------------------------|
|              | $\mathcal{M}_{\text{global-3}}^{\text{FCNN}}$ | $\mathcal{M}_{\text{global-3}}^{\text{GCN}}$ | $\mathcal{M}_{\text{global-3}}^{\text{CHC}}$ | $\mathcal{M}_{\text{global-3}}^{\text{SC}}$ | $\mathcal{M}_{\text{global-3}}^{\text{GC}}$ | $\mathcal{M}_{\text{global-3}}^{\text{GAT}}$ |
| 24-ieee-rtts | $0.18 \pm 0.02$                               | $2.48 \pm 0.12$                              | $0.69 \pm 0.05$                              | $0.89 \pm 0.07$                             | $1.71 \pm 0.34$                             | $2.78 \pm 0.18$                              |
| 30-ieee      | $0.05 \pm 0.01$                               | $1.41 \pm 0.28$                              | $0.08 \pm 0.01$                              | $0.11 \pm 0.03$                             | $0.51 \pm 0.12$                             | $2.95 \pm 0.22$                              |
| 39-epri      | $0.89 \pm 0.10$                               | $4.44 \pm 0.12$                              | $2.42 \pm 0.05$                              | $2.41 \pm 0.14$                             | $4.86 \pm 0.95$                             | $4.75 \pm 0.29$                              |
| 57-ieee      | $0.52 \pm 0.11$                               | $1.91 \pm 0.15$                              | $1.25 \pm 0.13$                              | $1.31 \pm 0.13$                             | $1.67 \pm 0.15$                             | $2.29 \pm 0.16$                              |
| 73-ieee-rtts | $0.21 \pm 0.07$                               | $1.37 \pm 0.26$                              | $0.61 \pm 0.02$                              | $0.67 \pm 0.02$                             | $1.15 \pm 0.13$                             | $1.83 \pm 0.11$                              |
| 118-ieee     | $0.39 \pm 0.03$                               | $2.12 \pm 0.07$                              | $1.26 \pm 0.06$                              | $1.27 \pm 0.07$                             | $1.47 \pm 0.12$                             | $2.43 \pm 0.12$                              |
| 162-ieee-dtc | $2.61 \pm 0.10$                               | $3.75 \pm 0.11$                              | $3.07 \pm 0.09$                              | $2.87 \pm 0.13$                             | $3.55 \pm 0.22$                             | $4.84 \pm 0.22$                              |
| 300-ieee     | $2.06 \pm 0.06$                               | $3.96 \pm 0.16$                              | $2.42 \pm 0.05$                              | $2.35 \pm 0.07$                             | $3.19 \pm 0.23$                             | $3.59 \pm 0.24$                              |
| 588-sdet     | $2.56 \pm 0.06$                               | $3.66 \pm 0.07$                              | $3.18 \pm 0.05$                              | $3.21 \pm 0.08$                             | $10.21 \pm 2.51$                            | $5.01 \pm 0.24$                              |
| 1354-pegase  | $0.83 \pm 0.12$                               | $2.09 \pm 0.11$                              | $1.43 \pm 0.09$                              | $1.36 \pm 0.09$                             | $2.64 \pm 0.11$                             | $2.51 \pm 0.14$                              |
| 2853-sdet    | $5.99 \pm 0.16$                               | $11.54 \pm 0.48$                             | $9.03 \pm 0.29$                              | $8.35 \pm 0.13$                             | $13.98 \pm 0.44$                            | $11.15 \pm 0.59$                             |

TABLE V

MSE STATISTICS (MEAN AND TWO-SIDED 95% CONFIDENCE INTERVALS) OF THE TEST SETS FOR LOCAL AND EXTENDED GLOBAL REGRESSION GNN MODELS USING ADMITTANCE MATRIX (FIXED TOPOLOGY)

| Case         | MSE ( $\times 10^{-3}$ )                    |                                             |                                             |                                              |                                              |                                              |
|--------------|---------------------------------------------|---------------------------------------------|---------------------------------------------|----------------------------------------------|----------------------------------------------|----------------------------------------------|
|              | $\mathcal{M}_{\text{local-3}}^{\text{GCN}}$ | $\mathcal{M}_{\text{local-3}}^{\text{CHC}}$ | $\mathcal{M}_{\text{local-3}}^{\text{GAT}}$ | $\mathcal{M}_{\text{global-4}}^{\text{GCN}}$ | $\mathcal{M}_{\text{global-4}}^{\text{CHC}}$ | $\mathcal{M}_{\text{global-4}}^{\text{GAT}}$ |
| 24-ieee-rtts | $60.26 \pm 0.53$                            | $25.89 \pm 0.14$                            | $67.83 \pm 9.26$                            | $2.16 \pm 0.08$                              | $0.46 \pm 0.04$                              | $2.56 \pm 0.15$                              |
| 30-ieee      | $8.67 \pm 1.05$                             | $0.52 \pm 0.14$                             | $28.47 \pm 9.82$                            | $1.17 \pm 0.38$                              | $0.11 \pm 0.02$                              | $2.85 \pm 0.22$                              |
| 39-epri      | $16.12 \pm 6.49$                            | $3.86 \pm 0.16$                             | $13.94 \pm 2.79$                            | $3.14 \pm 0.19$                              | $2.21 \pm 0.08$                              | $3.08 \pm 0.22$                              |
| 57-ieee      | $4.85 \pm 0.21$                             | $2.25 \pm 0.37$                             | $8.87 \pm 3.25$                             | $1.75 \pm 0.14$                              | $1.26 \pm 0.21$                              | $2.41 \pm 0.22$                              |
| 73-ieee-rtts | $43.09 \pm 6.61$                            | $31.58 \pm 0.04$                            | $57.05 \pm 3.62$                            | $0.88 \pm 0.03$                              | $0.33 \pm 0.03$                              | $2.32 \pm 1.33$                              |
| 118-ieee     | $25.37 \pm 4.74$                            | $7.75 \pm 0.19$                             | $35.44 \pm 1.51$                            | $2.65 \pm 0.11$                              | $1.45 \pm 0.08$                              | $4.66 \pm 0.26$                              |
| 162-ieee-dtc | $11.19 \pm 0.18$                            | $8.29 \pm 0.16$                             | $11.51 \pm 0.13$                            | $4.12 \pm 0.16$                              | $3.33 \pm 0.11$                              | $5.95 \pm 1.12$                              |
| 300-ieee     | $11.56 \pm 0.46$                            | $9.51 \pm 0.07$                             | $78.56 \pm 9.67$                            | $4.35 \pm 0.17$                              | $2.71 \pm 0.06$                              | $5.29 \pm 1.63$                              |
| 588-sdet     | $21.11 \pm 1.15$                            | $16.28 \pm 0.19$                            | $28.56 \pm 8.91$                            | $3.87 \pm 0.06$                              | $3.83 \pm 0.12$                              | $71.49 \pm 9.76$                             |

TABLE VI

NUMBER OF PARAMETERS FOR GLOBAL CLASSIFICATION MODELS (VARYING TOPOLOGY)

| Case         | # of parameters                               |                                               |                                              |                                              |                                              |                                             |                                             |
|--------------|-----------------------------------------------|-----------------------------------------------|----------------------------------------------|----------------------------------------------|----------------------------------------------|---------------------------------------------|---------------------------------------------|
|              | $\mathcal{M}_{\text{global-3}}^{\text{FCNN}}$ | $\mathcal{M}_{\text{global-1}}^{\text{FCNN}}$ | $\mathcal{M}_{\text{global-4}}^{\text{GCN}}$ | $\mathcal{M}_{\text{global-3}}^{\text{GCN}}$ | $\mathcal{M}_{\text{global-3}}^{\text{CHC}}$ | $\mathcal{M}_{\text{global-3}}^{\text{SC}}$ | $\mathcal{M}_{\text{global-3}}^{\text{GC}}$ |
| 24-ieee-rtts | 14372                                         | 4263                                          | 2067                                         | 4324                                         | 4804                                         | 4964                                        | 4484                                        |
| 30-ieee      | 4740                                          | 915                                           | 1083                                         | 700                                          | 1180                                         | 1340                                        | 860                                         |
| 39-epri      | 13661                                         | 4345                                          | 3283                                         | 2435                                         | 2915                                         | 3075                                        | 2595                                        |
| 57-ieee      | 17233                                         | 3680                                          | 3180                                         | 2091                                         | 2571                                         | 2731                                        | 2251                                        |
| 73-ieee-rtts | 77552                                         | 25431                                         | 20137                                        | 24455                                        | 24935                                        | 25095                                       | 24615                                       |
| 118-ieee     | 112037                                        | 34839                                         | 31311                                        | 35597                                        | 37421                                        | 38029                                       | 36205                                       |
| 162-ieee-dtc | 171139                                        | 47450                                         | 42782                                        | 48208                                        | 50032                                        | 50640                                       | 48816                                       |
| 300-ieee     | 600416                                        | 169482                                        | 158790                                       | 170240                                       | 172064                                       | 172672                                      | 170848                                      |
| 588-sdet     | 1866920                                       | 423720                                        | 409908                                       | 434558                                       | 436382                                       | 436990                                      | 435166                                      |
